# Supplementary material for: Byzantine Fault-Tolerant Distributed Machine Learning Using Stochastic Gradient Descent (SGD) and Norm-Based Comparative Gradient Elimination (CGE)
Source: arXiv:2008.04699 source file (2021-04-18)
Supplement: Supplementary file 1 [file appendix_experiments.tex]

\section{Supplemental experiments}

In this section, we present supplemental results of experiments that we have conducted.

\subsection{Experiments with no filter}
\label{sub:exp-with-no-filter}

As a complement to plots in Section \ref{ssub:frac-of-faults}, we include a group of results here documenting the performance of SGD with no filter when facing different fractions of fault agents in the system. Figure~\ref{fig:fault-fraction-5} presents such results. As is shown in Figure~\ref{fig:fault-fraction-5}(a), (b) and (e), for these three types of faults, \textit{reverse}, \textit{coordinate-wise}, and \textit{random}, even only 1 out of 10 agents being fault (or 10\%), it would lead to no convergence at all. On the other hand, \textit{norm-confusing}, shown in Figure~\ref{fig:fault-fraction-5}(c), can be relatively easy, which only slow down the convergence speed of SGD, even if no filter is applied. Also, \textit{label-flipping}, shown in Figure~\ref{fig:fault-fraction-5}(d), is also a `easier' fault, that has similar convergence speed to fault-free case, but will lead to a suboptimal value.

\begin{figure}[t]
    \centering
    \includegraphics[width=\textwidth]{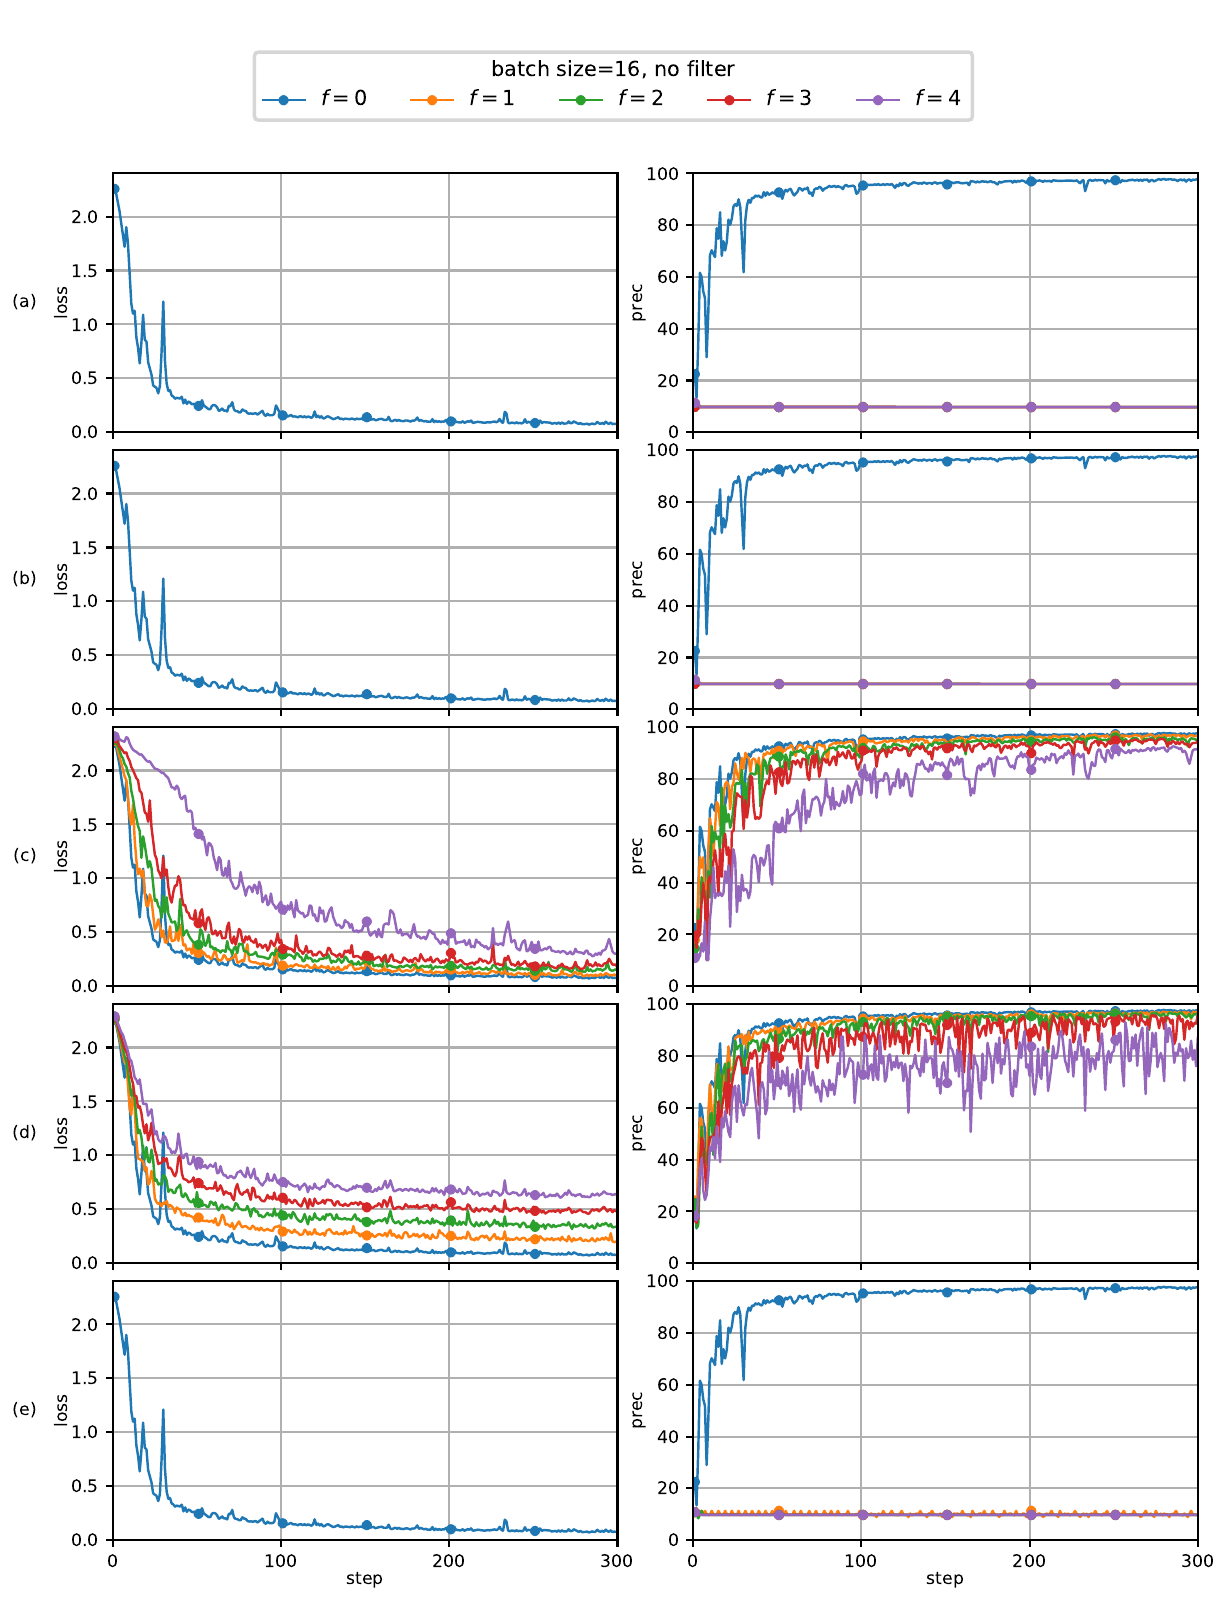}
    \caption{Comparison among different numbers of fault agents. No filter is used but plain averaging, with batch size be 16. Different row presents different fault types: (a) \textit{reverse}, (b) \textit{coordinate-wise}, (c) \textit{norm-confusing}, (d) \textit{label-flipping}, and (e) \textit{random}.}
    \label{fig:fault-fraction-5}
\end{figure}
