# Supplementary material for: Byzantine Fault-Tolerant Distributed Machine Learning Using Stochastic Gradient Descent (SGD) and Norm-Based Comparative Gradient Elimination (CGE)
Source: arXiv:2008.04699 source file (2021-04-18)
Supplement: Supplementary file 2 [file supplementary_experiments.tex]

\section{Additional Experimental Results}
\label{sec:add_exp}

Other than the results we shown in the paper, experiments under various parameter settings are also conducted. Here we present the results.

% Next, we present the remaining details and outcomes of our experiments.
\subsection{Experiments with MNIST dataset}
\begin{figure}[b!]
    \centering
    \begin{subfigure}{\textwidth}
        \includegraphics[width=\textwidth]{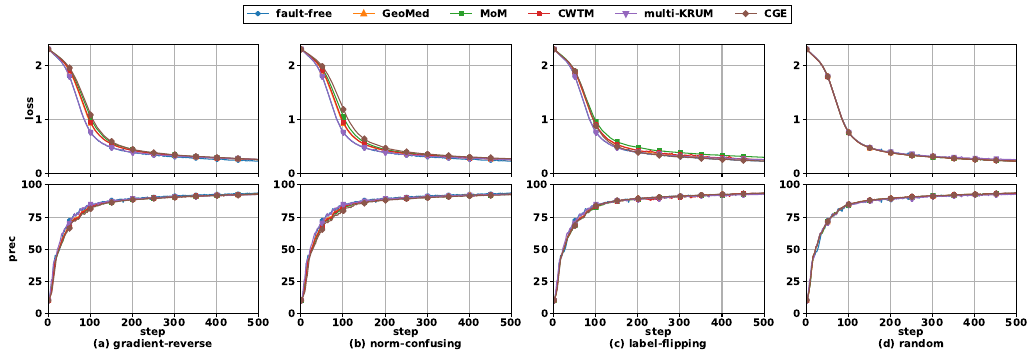}
        \caption{$f=4$}
        \label{fig:fault-40-4}
    \end{subfigure}\\
    \begin{subfigure}{\textwidth}
        \includegraphics[width=\textwidth]{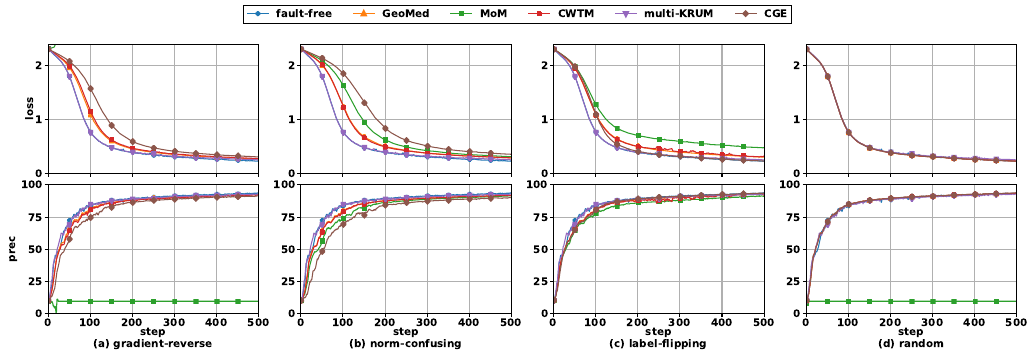}
        \caption{$f=8$}
        \label{fig:fault-40-8}
    \end{subfigure}\\
    \begin{subfigure}{\textwidth}
        \includegraphics[width=\textwidth]{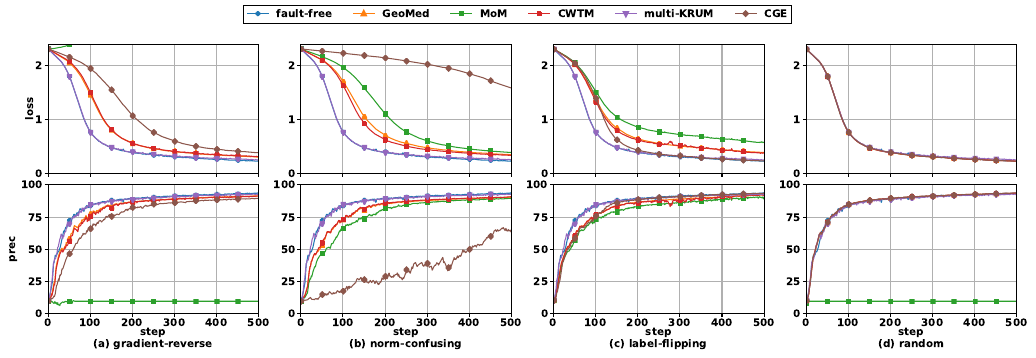}
        \caption{$f=12$}
        \label{fig:fault-40-12}
    \end{subfigure}
    \caption{\footnotesize Distributed learning of the convolutional neural network $\mathsf{LeNet}$ for the MNIST dataset using the D-SGD method with different gradient-filters (represented by different colors) to tolerate different numbers of faulty agents in the system. The training losses and the testing precisions evaluated by the server after $0$ to $500$ iterations (or steps) of the different learning algorithms are plotted in the first and the second rows, respectively. Different columns contain the results for different types of faults simulated by the faulty agents. Here, the data batch size $k=64$.}
    \label{fig:mnist-fault-comparison-01}
\end{figure}

We conducted series of experiments with MNIST dataset and 40 agents in the system while changing the number of faulty agents in the system from 1 to 12. Here we selectively present results with $f=4,\,8$, and $12$, or $10\%,\,20\%$, and $30\%$ of faulty agents in the system respectively, shown in Figure~\ref{fig:mnist-fault-comparison-01}. Note that theoretically, MoM with $b=2$ can only tolerate less than 8 fault agents in a 40-agent system, which is also supported by some experimental results.\\ 

We also observe that \textit{norm-confusing} is a difficult fault type for CGE, as its performance deteriorates fast when number of faulty agents increases, comparing to its performances when facing other fault types, which are comparable to other state-of-the-art gradient filters no matter how many faulty agents. Need to note that when facing \textit{norm-confusing}, instead of being unable to converge, CGE only converges slower.

\subsection{Experiments with CIFAR-10 dataset}

\begin{figure}[tb!]
    \centering
    \includegraphics[width=\linewidth]{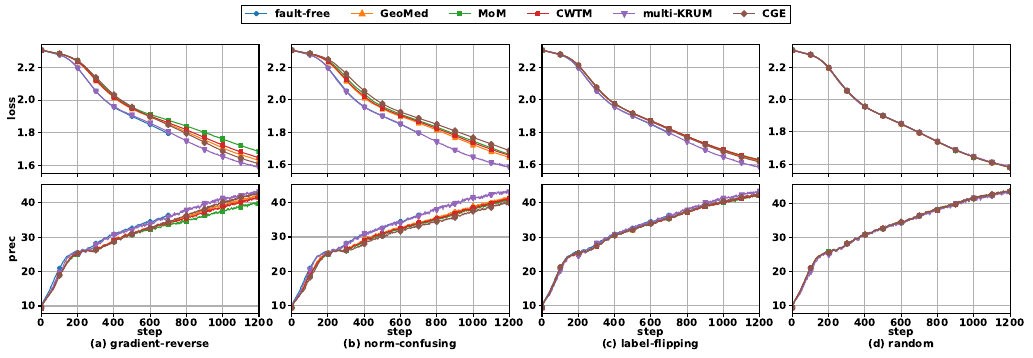}
    \caption{Distributed learning of $\mathsf{LeNet}$ for CIFAR-10 dataset using the D-SGD method with batch size $k=64$ and the different gradient-filters (represented using different colors) in the presence of $f = 4$ faulty agents exhibiting different Byzantine faults.}
    \label{fig:cifar-fault-comparison-01}
\end{figure}

\begin{figure}[tb!]
    \centering
    \includegraphics[width=0.6\linewidth]{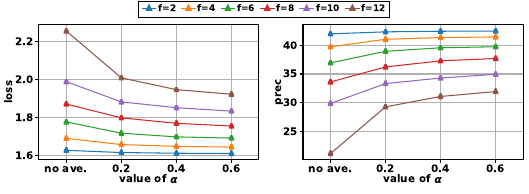}
    \caption{Average training losses and testing precisions evaluated between $1175$ to $1200$ steps of the D-SGD method with CGE gradient-filter for distributed learning of the neural network $\mathsf{LeNet}$ (for the CIFAR-10 dataset) in the presence of different number of faulty agents $f$ (represented by different colors) when applying temporal averaging of stochastic for different values of $\alpha$. \emph{no ave.} indicates the case when no averaging is not used. Here, the data batch-size $k = 64$.}
    \label{fig:cifar-averaging-01}
\end{figure}

We further conducted our experiments with CIFAR-10 dataset and 40 agents in the system. We trained an extra 700 steps with batch size $k=64$ and $f=4$ faulty agents in the system, with results shown in Figure~\ref{fig:cifar-fault-comparison-01}. We also applied our proposed temporal averaging scheme. As is shown in Figure~\ref{fig:cifar-averaging-01}, with temporal averaging scheme, for classification task on CIFAR-10 dataset, better performance can be achieved as well, if trained with same number of steps.\\
