# Supplementary material for: Byzantine Fault-Tolerant Distributed Machine Learning Using Stochastic Gradient Descent (SGD) and Norm-Based Comparative Gradient Elimination (CGE)
Source: arXiv:2008.04699 source file (2021-04-18)
Supplement: Supplementary file 4 [file supplementary_proof.tex]

\documentclass[letterpaper, 11pt]{article}

\usepackage{geometry}
\geometry{top = 1 in, bottom = 1 in, left=1.5 in, right=1.5 in}

% if you need to pass options to natbib, use, e.g.:
%     \PassOptionsToPackage{numbers, compress}{natbib}
% before loading neurips_2020

% ready for submission
% \usepackage{neurips_2020}

% to compile a preprint version, e.g., for submission to arXiv, add add the
% [preprint] option:
%     \usepackage[preprint]{neurips_2020}

% to compile a camera-ready version, add the [final] option, e.g.:
%     \usepackage[final]{neurips_2020}

% to avoid loading the natbib package, add option nonatbib:
    %  \usepackage[nonatbib]{neurips_2020}

\usepackage[utf8]{inputenc} % allow utf-8 input
\usepackage[T1]{fontenc}    % use 8-bit T1 fonts
\usepackage{hyperref}       % hyperlinks
\usepackage{url}            % simple URL typesetting
\usepackage{booktabs}       % professional-quality tables
\usepackage{amsfonts}       % blackboard math symbols
\usepackage{nicefrac}       % compact symbols for 1/2, etc.
\usepackage{microtype}      % microtypography
\usepackage[toc]{appendix}
\usepackage[ruled,vlined]{algorithm2e}
\usepackage{setspace}

\usepackage{amsmath,amssymb}
\usepackage{amsthm}
\usepackage{amssymb,graphicx,verbatim,enumitem,mdframed,mathrsfs}
\usepackage{mdframed}
\usepackage{subcaption}
\usepackage[toc]{appendix}

% % \usepackage{algorithm2e}
% \usepackage{algorithm}
% \usepackage{algorithmic}
\usepackage{arydshln}

\captionsetup{font=footnotesize}
%\captionsetup[sub]{font=small}

%\usepackage{minipage}     % allow multiple figures in a line
%\usepackage{subfigure}

% \newtheorem{theorem}{\textbf{Theorem}}
% \newtheorem{corollary}{\textbf{Corollary}}
% \newtheorem{lemma}{\textbf{Lemma}}

\newtheorem*{theorem*}{\bfseries Theorem}
\newtheorem{theorem}{\bfseries Theorem}

\newtheorem{corollary}{\bfseries Corollary}

\newtheorem*{lemma*}{\bfseries Lemma}

\newtheorem{assumption}{\bfseries Assumption}

\providecommand{\iprod}[2]{\ensuremath{\left\langle #1,\,#2  \right\rangle}}
\providecommand{\norm}[1]{\ensuremath{\left\lVert#1\right\rVert }}

\def\E{\mathbb{E}}
\def\R{\mathbb{R}}
\def\D{\mathcal{D}}

\def\z{{\bf z}}
\def\M{\mathsf{M}}

\def\var{\mathsf{Var}}

\def\H{\mathcal{H}}

\title{\bf Supplementary File: \\Proofs and Additional Empirical Results}
% \title{Fault-Tolerance in Distributed Machine Learning by\\ Robustifying Distributed Stochastic Gradient Descent}
% \textcolor{red}{++++++++++ need to revise title ++++++++++++++++++++}}

% % \author{...}
\author{Anonymous Authors}
\date{\it (Paper Title) Byzantine Fault-Tolerant Distributed Machine Learning Using SGD And Norm-Based Comparative Gradient Elimination (CGE)}

% \pagenumbering{roman}

\begin{document}

\maketitle

\noindent
This supplementary file contains the following:
\begin{itemize}
    \item Formal proofs of Theorem 1 and Corollary 1
    \item Additional experimental results.
\end{itemize}
The formal proofs are presented in Sections~\ref{sec:review} and~\ref{app:pf_thm}. The additional experimental results are presented in Section~\ref{sec:add_exp}.\\

\noindent For convenience, we review our proposed algorithm below. 

\begin{algorithm}[htb!]
\SetAlgoLined
Steps in each iteration $t$. 
\\~\\

\noindent $\diamond ~$ {\bf Step S1}: The server broadcasts the current estimate $w^{t}$ to all the agents.
\\~\\

% 
% \\~\\

The gradient received by the server from agent $i$ is denoted as $g_i^t$. 
\\~\\
% Each non-faulty agent $i$ will then send to the server a stochastic gradient of the global expected loss function $Q(w)$ at $w^t$, i.e., a noisy estimator of the gradient $\nabla Q(w^t)$. A faulty agent may send an incorrect arbitrary vector for its stochastic gradient.
% If no gradient is received from some agent $i$, then agent $i$ must
% be faulty (because the system is assumed to be synchronous) -- in this case, the server assumes a default value of {\bf 0} vector for the missing gradient $g_i^t$.
% \\~\\
    
\noindent $\diamond ~$ {\bf Step S2 (CGE gradient-filter):} The server sorts the $n$ received gradients as follows: 
\begin{align}
    \norm{g^t_{i_1}} \leq \ldots \leq \norm{ g^t_{i_{n-f}}} \leq \norm{ g^t_{i_{n-f+1}}} \leq \ldots \leq \norm{g^t_{i_{n}}}. \label{eqn:order}
\end{align}
Gradient with the $j$-th smallest norm, $g^t_{i_j}$, is received from agent $i_j$. 
\\~\\

The server updates its current estimate using only $n-f$ stochastic gradients with smallest $n-f$ norms as shown below. 
\begin{align}
    w^{t+1} = w^t - \eta_t \, \sum_{j = 1}^{n-f} g^t_{i_j} \label{eqn:algo_1}
\end{align}
where $\eta_t$ is the {\em step-size} of iteration $t$.

\caption{D-SGD with CGE Gradient-filter}
\label{alg:cge}
\end{algorithm}%

To {\bf compute a stochastic gradient} in each iteration $t$, each non-faulty agent $i$ samples
% To compute correct stochastic gradients of the global expected loss function $Q(w)$, in each iteration $t$ each non-faulty agent $i$ samples 
$k$ data points $\{z^t_{i_1}, \ldots, \, z^t_{i_k}\}$ i.i.d.~from the data-generating distribution $\D$. 
% As elaborated below in Section~\ref{sub:ft}, the average of the gradients of the loss functions $\ell(w, \, z^t_{i_j}), ~ j = 1, \ldots, \, k$, with respect to $w$ is an unbiased noisy estimator of the true gradient $\nabla Q(w)$, and can be used as a stochastic gradient of $Q(w)$. 
Specifically, each non-faulty agent $i$ computes a stochastic gradient 
\begin{align}
    g^t_i = \frac{1}{k} \sum_{j = 1}^k \nabla \ell(w^t, \, z^t_{i_j}), \quad \forall t. \label{eqn:avg_grad}
\end{align}
~

Upon reviewing the fault-tolerance guarantee for our algorithm below in Section~\ref{sec:review}, we present a formal proof of Theorem 1 in Section~\ref{app:pf_thm}. Proof of Corollary 1 is presented in Section~\ref{sec:review} below. Later, in Section~\ref{sec:add_exp}, we present some additional empirical results.

\section{Review of the Fault-Tolerance Property}
\label{sec:review}

We restate below our notation and assumptions from the main paper.

\begin{itemize}
    \item For each non-faulty agent $i$, let 
    \begin{align}
        \z^t_i = \{z^t_{i_1}, \ldots, \, z^t_{i_k}\} \label{eqn:non-f_data}
    \end{align}
    denote the collection i.i.d.~data points sampled by the agent $i$ in iteration $t$. Now, for each agent $i$ and iteration $t$ we define a random variable 
    \begin{align}
        \zeta^t_i = \left\{ \begin{array}{ccc} \z^t_i & , & \text{agent $i$ is non-faulty} \\ g^t_i & , & \text{agent $i$ is faulty}\end{array}\right. \label{eqn:def_zeta_i}
    \end{align}
    Recall that~$g^t_i$ may be an arbitrary $d$-dimensional random variable for each Byzantine faulty agent $i$. For each iteration $t$, let
    \begin{align}
        \zeta^t = \{\zeta^t_i, ~ i = 1, \ldots, \, n\}, \label{eqn:def_zeta}
    \end{align}
    and let $\E_t$ denote the expectation of a function of the collective random variables $\zeta^0, \ldots, \, \zeta^t$, given the initial estimate $w^0$. Specifically, 
    \begin{align}
        \E_t(\cdot) = \E_{\zeta^0, \ldots, \, \zeta^{t}} (\cdot), \quad \forall t \geq 0. \label{eqn:notation_exp}
    \end{align}
    \item We define a {\em fault-tolerance margin}  
    \begin{align}
        \alpha = \frac{\lambda}{2\lambda + \mu} - \frac{f}{n} \label{eqn:alpha_learn}
    \end{align}
    that determines the maximum fraction of faulty agents $f/n$ tolerable by our algorithm. Lastly, we define an upper bound for the step-size in~\eqref{eqn:algo_1},
    \begin{align}
        \overline{\eta} = \left(\frac{2(2 \lambda + \mu)n}{n^2 + (n-f)^2 \mu^2 } \right) \, \alpha. \label{eqn:step_learn}
    \end{align}
    % \item Let
    % \begin{align}
    %     \M^2 = \left(\frac{f^2 \left( 1 + \sqrt{n-f-1}\right)^2}{n^2} + \eta^2 (n-f)^2 \right) \sigma^2. \label{eqn:ss_error}
    % \end{align}
\end{itemize}
~

% Our assumptions are re-stated below.

% \[Z^t_1 ~ Z^t_2 ~ Z^t_n\]
% denote the collection of $k$ data points for iteration $t$ where each data point is chosen .  that in step S1 each iteration $t$, a non-faulty agent $i$ independently chooses a data point $z^t_i$ from probability distribution $\D$, and sends a {\em stochastic} gradient $g^t_i = \nabla \ell (w^t; z^t_i)$. As $Q(w) = \E_{z \sim \D} ~ \ell (w; z), ~ \forall w$, for every non-faulty agent $i$, 
% \[\E_{z^t_i \sim \D} ~ ( g^t_i ) = \nabla Q(w^t), \quad \forall t.\]

\begin{assumption}[Bounded variance]
\label{asp:bnd_var}
For each non-faulty agent $i$, assume that the variance of $g^t_i$ is bounded. Specifically, there exists a finite real value $\sigma$ such that for all non-faulty agent $i$,
\[\E_{\zeta^t_i} \norm{ g^t_i - \E_{\zeta^t_i} \left(g^t_i\right)}^2 \leq \sigma^2, \quad \forall t.\]
\end{assumption}

% As stated below, we also assume that the gradient of the expected loss function $\nabla Q(w)$ is Lipschitz continuous, and that the function $Q(w)$ is strongly convex~\cite{bottou2018optimization}. 

\begin{assumption}[Lipschitz continuity of gradients]
\label{asp:lip}
Assume that there exists a finite positive real value $\mu$ such that for all $w, \, w' \in \R^d$,
\begin{align*}
    \norm{\nabla Q(w) - \nabla Q(w')} \leq \mu \norm{w - w'}.
\end{align*}
\end{assumption}

\begin{assumption}[Strong convexity]
\label{asp:str_cvx}
Assume that there exists a finite positive real value $\lambda$ such that for all $w, \, w' \in \R^d$,
\begin{align*}
    \iprod{w - w'}{\nabla Q(w) - \nabla Q(w')} \geq \lambda \norm{w - w'}^2.
\end{align*}
\end{assumption}

% As noted by~\cite{bottou2018optimization}, the assumption on strong convexity of $Q(w)$ is not very restrictive in the practical scenarios of machine learning. For instance, in many situations when a convex learning model is used -- such as logistic regression or support vector machine -- it is often regularized by a strongly
% convex function. Moreover, even if the global cost $Q(w)$ is not strongly convex over the entire search space $\R^d$, it is so in the neighborhood of local minimizers. This means that our algorithm can guarantee fault-tolerance in small regions of the learning parameter search space.\\

We re-state below Theorem~\ref{thm:conv}, a key result on the fault-tolerance of our algorithm. Recall that $w^*$ denotes a minimum of the global expected loss function $Q(w)$, i.e., 
\[w^* \in \arg \min_w Q(w).\]
% The convergence of the modified algorithm presented in Section~\ref{sec:learn} is in expectation, where the notation $\E \norm{w^t - w^*}^2$ denotes the joint expectation of $\norm{w^t - w^*}^2$ over all the data points chosen by non-faulty agents up to the $t$-th iteration. That is, if $z^t$ denotes the random data points chosen by all the agents (including the faulty agents) for iteration $t$, then

% Let,
% \begin{align}
%     \eta < \overline{\eta} = \frac{2(2 \lambda + \mu)n}{n^2 + (n-f)^2 \mu^2 } \, \alpha, \label{eqn:step_learn}
% \end{align}
% then $\E \norm{w^{t} - w^*}^2$ converges linearly in the proximity of $w^*$ with rate of convergence 
% \[\rho = 1 - 2 \eta (2 \lambda + \mu) \alpha n + \eta^2 \left(n^2 + (n-f)^2 \mu^2 \right).\]
% Specifically, we obtain the following convergence result.\\

% \noindent \fbox{\begin{minipage}{0.96\textwidth}
\begin{theorem}[Restated]
\label{thm:conv}
Consider Algorithm~\ref{alg:cge}. Suppose that the Assumptions~\ref{asp:bnd_var},~\ref{asp:lip}, and~\ref{asp:str_cvx} hold true. If the fault-tolerance margin $\alpha$ is positive, and in the update law~\eqref{eqn:algo_1} the step-size $\eta_t = \eta \in \left(0, ~ \overline{\eta} \right)$ for all $t$ then 
\begin{align}
    \rho  = 1 - \left(n^2 + (n-f)^2 \mu^2 \right) \, \eta \left( \overline{\eta} - \eta \right) \in (0, ~ 1), \label{eqn:rho}
\end{align}
and, for all $t \geq 1$, 
\begin{align}
    \E_{t-1} \norm{w^{t} - w^*}^2 \leq \rho^{t} \norm{w^{0} - w^*}^2 + \left(\frac{1 - \rho^{t}}{ 1- \rho}\right) \M^2 \label{eqn:rate}
\end{align}
where
\begin{align}
    \M^2 = \left(\frac{f^2 \left( 1 + \sqrt{n-f-1}\right)^2}{n^2} + \eta^2 (n-f)^2 \right) \sigma^2. \label{eqn:ss_error}
\end{align}
% \begin{align}
%     \rho  = 1 - \left(n^2 + (n-f)^2 \mu^2 \right) \, \eta \left( \overline{\eta} - \eta \right)  \label{eqn:rho}
% \end{align}
% has a positive value less than $1$, and for all $t \geq 0$,
% \begin{align}
%     \E_{t} \norm{w^{t+1} - w^*}^2 \leq \rho^{t+1} \norm{w^{0} - w^*}^2 + \left(\frac{1 - \rho^{t+1}}{ 1- \rho}\right) \M^2.\label{eqn:rate}
% \end{align}
% where $w^*$ is as defined in~\eqref{eqn:obj}.
% $$ \rho_f(\eta) = 1 - \eta n \, \left(2 (\lambda + 2\mu) \alpha - \eta n \mu^2 \right) \in [0, 1), \text{ and } $$
\end{theorem}

Before we proceed to our proof of Theorem~\ref{thm:conv}, we restate below Corollary~\ref{cor:learn} along with its proof. Recall that notation $Pr(\cdot)$ denotes the probability of an event. 

% \noindent \fbox{\begin{minipage}{0.96\textwidth}
\begin{corollary}[Restated]
\label{cor:learn}
Consider our iterative algorithm. If the conditions stated in Theorem~\ref{thm:conv} hold true then
% tu Assumptions~\ref{asp:bnd_var}-\ref{asp:str_cvx} hold true, the fault-tolerance margin $\alpha$ is positive, and the step-size $\eta_t$ in~\eqref{eqn:algo_1} has a constant positive real value $\eta$ for all $t$. If $\eta < \overline{\eta}$ then 
for every positive real value $\epsilon$,
\[\lim_{t \to \infty} Pr \left( \norm{w^t - w^*}^2 \leq \epsilon \right) \geq 1 - \frac{1}{\epsilon} ~ \left( \frac{\M^2}{1 - \rho}\right). \]
\end{corollary}
\begin{proof}
Note, from Markov's inequality~\cite{mohri2018foundations}, that for an arbitrary positive real value $\epsilon$,
\begin{align}
    Pr \left( \norm{w^{t+1} - w^*}^2 \geq \epsilon \right) \leq \frac{\E_{t} \norm{w^{t+1} - w^*}^2 }{\epsilon}, \quad \forall t \geq 0. \label{eqn:markov}
\end{align}
If the conditions in Theorem~\ref{thm:conv} hold true then for all $t \geq 0$,
\begin{align*}
    \E_{t} \norm{w^{t+1} - w^*}^2 \leq \rho^{t+1} \norm{w^{0} - w^*}^2 + \left(\frac{1 - \rho^{t+1}}{ 1- \rho}\right) \M^2
\end{align*}
where $\rho \in (0, \, 1)$. Substituting from above in~\eqref{eqn:markov} we obtain, for all $t \geq 0$, that
\[ Pr \left( \norm{w^{t+1} - w^*}^2 \geq \epsilon \right) \leq \frac{1}{\epsilon} \left(\rho^{t+1} \norm{w^{0} - w^*}^2 + \left(\frac{1 - \rho^{t+1}}{ 1- \rho}\right) \M^2 \right).\]
Equivalently, 
\[Pr \left( \norm{w^{t+1} - w^*}^2 \leq \epsilon \right) \geq 1 - \frac{1}{\epsilon} \left(\rho^{t+1} \norm{w^{0} - w^*}^2 + \left(\frac{1 - \rho^{t+1}}{ 1- \rho}\right) \M^2 \right).\]
As $\rho < 1$, $\lim_{t \to \infty} \rho^t = 0$. Therefore, limiting $t$ to infinity on both sides of the above inequality proves the corollary, i.e.,
\[ \lim_{t \to \infty} Pr \left( \norm{w^{t} - w^*}^2 \leq \epsilon \right) \geq  1 -  \frac{1}{\epsilon}\left(\frac{\M^2}{ 1- \rho}\right).\]
\end{proof}

Our formal proof of Theorem~\ref{thm:conv} is presented in the subsequent section.

% \subsection{Proof of Theorem}
% Note, from~\eqref{eqn:algo_1}, that for each iteration $t$ the updated estimate $w^{t+1}$ is a function of the current estimate $w^t$, and the random variables $g^t_1, \ldots, \, g^t_n$. In case agent $i$ is non-faulty, recall from~\eqref{eqn:avg_grad} that the stochastic gradient $g^t_i$ is a function of $w^t$ and the collection of $k$ data points 
% \begin{align}
%     \z^t_i = \{z^t_{i_1}, \ldots, \, z^t_{i_k}\} \label{eqn:non-f_data}
% \end{align}
% that are independent and identically distributed (i.i.d.) by $\D$. In case agent $i$ is faulty, then $g^t_i$ is an arbitrary $d$-dimensional random variable. For each $i = 1, \ldots, \, n$, we define a random variable 
% \begin{align}
%     \zeta^t_i = \left\{ \begin{array}{ccc} \z^t_i & , & \text{$i$ is non-faulty} \\ ~\\ g^t_i & , & \text{$i$ is faulty}\end{array}\right. \label{eqn:def_zeta_i}
% \end{align}
% Let, 
% \begin{align}
%     \zeta^t = \left\{\zeta^t_1, \ldots, \, \zeta^t_n \right\}. \label{eqn:def_zeta}
% \end{align}
% ~

% For each agent $i$ and each iteration $t$, let $\E_{\zeta^t_i}(\cdot)$ denote the expected value of a function of the random variable $\zeta^t_i$ given the current estimate $w^t$. Similarly, for each non-faulty agent $i$, let $\E_{\z^t_i}(\cdot)$ denote the expected value of a function of the random variable $\z^t_i$ given the estimate $w^t$.\\

\input{conv_proof}

In the subsequent section, we present our additional empirical results.

\newpage

% Recall that the global expected loss function is defined to be
% \begin{align}
%     Q(w) = \underset{z \sim \D}{\E} \, \ell(w, \,z), \quad \forall w \in \R^d. \label{eqn:exp_loss}
% \end{align}

\section{Additional Experimental Results}
\label{sec:add_exp}

Other than the results we shown in the paper, experiments under various parameter settings are also conducted. Here we present the results.

% Next, we present the remaining details and outcomes of our experiments.
\subsection{Experiments with MNIST dataset}
\begin{figure}[b!]
    \centering
    \begin{subfigure}{\textwidth}
        \includegraphics[width=\textwidth]{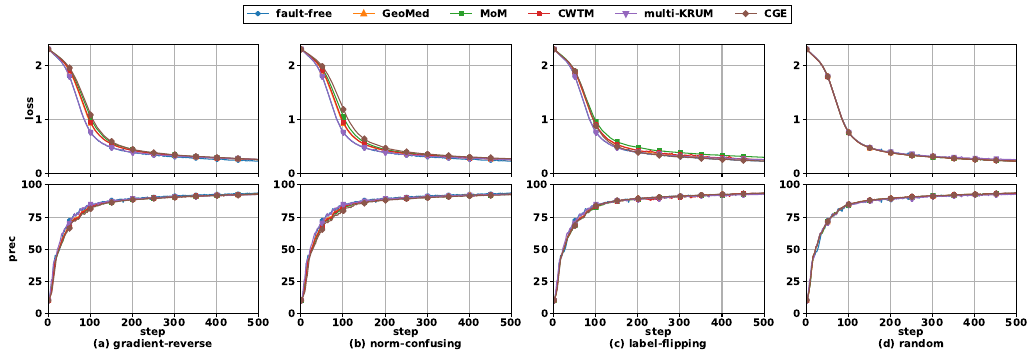}
        \caption{$f=4$}
        \label{fig:fault-40-4}
    \end{subfigure}\\
    \begin{subfigure}{\textwidth}
        \includegraphics[width=\textwidth]{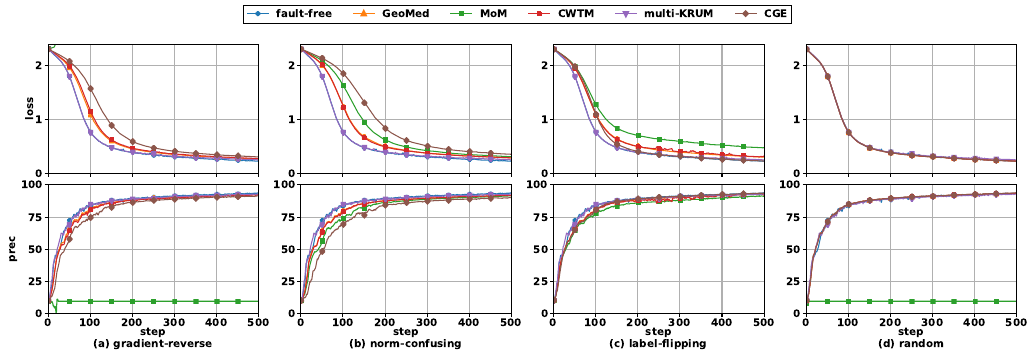}
        \caption{$f=8$}
        \label{fig:fault-40-8}
    \end{subfigure}\\
    \begin{subfigure}{\textwidth}
        \includegraphics[width=\textwidth]{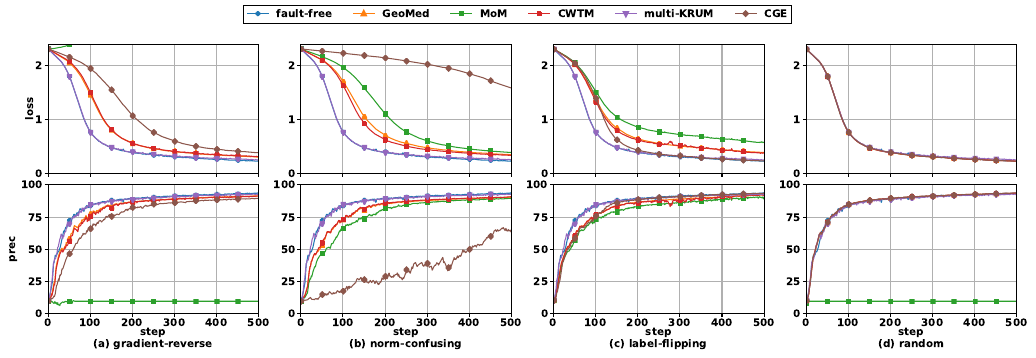}
        \caption{$f=12$}
        \label{fig:fault-40-12}
    \end{subfigure}
    \caption{\footnotesize Distributed learning of the convolutional neural network $\mathsf{LeNet}$ for the MNIST dataset using the D-SGD method with different gradient-filters (represented by different colors) to tolerate different numbers of faulty agents in the system. The training losses and the testing precisions evaluated by the server after $0$ to $500$ iterations (or steps) of the different learning algorithms are plotted in the first and the second rows, respectively. Different columns contain the results for different types of faults simulated by the faulty agents. Here, the data batch size $k=64$.}
    \label{fig:mnist-fault-comparison-01}
\end{figure}

We conducted series of experiments with MNIST dataset and 40 agents in the system while changing the number of faulty agents in the system from 1 to 12. Here we selectively present results with $f=4,\,8$, and $12$, or $10\%,\,20\%$, and $30\%$ of faulty agents in the system respectively, shown in Figure~\ref{fig:mnist-fault-comparison-01}. Note that theoretically, MoM with $b=2$ can only tolerate less than 8 fault agents in a 40-agent system, which is also supported by some experimental results.\\ 

We also observe that \textit{norm-confusing} is a difficult fault type for CGE, as its performance deteriorates fast when number of faulty agents increases, comparing to its performances when facing other fault types, which are comparable to other state-of-the-art gradient filters no matter how many faulty agents. Need to note that when facing \textit{norm-confusing}, instead of being unable to converge, CGE only converges slower.

\subsection{Experiments with CIFAR-10 dataset}

\begin{figure}[tb!]
    \centering
    \includegraphics[width=\linewidth]{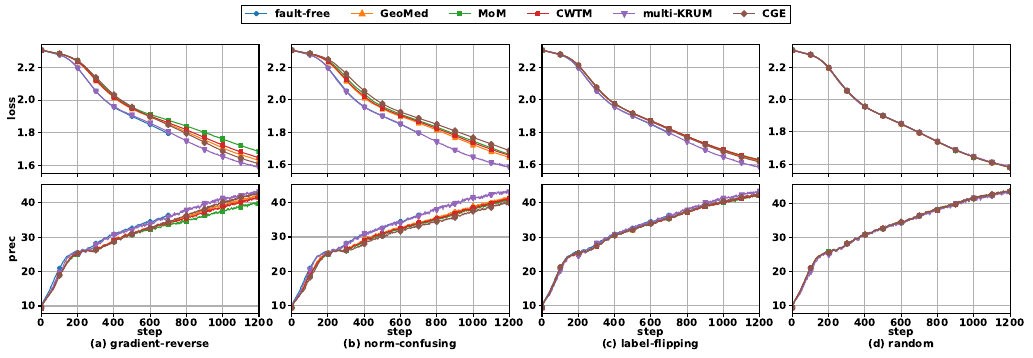}
    \caption{Distributed learning of $\mathsf{LeNet}$ for CIFAR-10 dataset using the D-SGD method with batch size $k=64$ and the different gradient-filters (represented using different colors) in the presence of $f = 4$ faulty agents exhibiting different Byzantine faults.}
    \label{fig:cifar-fault-comparison-01}
\end{figure}

\begin{figure}[tb!]
    \centering
    \includegraphics[width=0.6\linewidth]{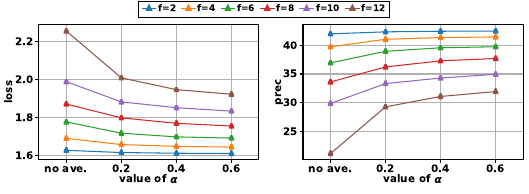}
    \caption{Average training losses and testing precisions evaluated between $1175$ to $1200$ steps of the D-SGD method with CGE gradient-filter for distributed learning of the neural network $\mathsf{LeNet}$ (for the CIFAR-10 dataset) in the presence of different number of faulty agents $f$ (represented by different colors) when applying temporal averaging of stochastic for different values of $\alpha$. \emph{no ave.} indicates the case when no averaging is not used. Here, the data batch-size $k = 64$.}
    \label{fig:cifar-averaging-01}
\end{figure}

We further conducted our experiments with CIFAR-10 dataset and 40 agents in the system. We trained an extra 700 steps with batch size $k=64$ and $f=4$ faulty agents in the system, with results shown in Figure~\ref{fig:cifar-fault-comparison-01}. We also applied our proposed temporal averaging scheme. As is shown in Figure~\ref{fig:cifar-averaging-01}, with temporal averaging scheme, for classification task on CIFAR-10 dataset, better performance can be achieved as well, if trained with same number of steps.\\

\bibliographystyle{plain}
\bibliography{ref.bib}

\appendix
\section{Proofs of Lemma~\ref{lem:bnd_norm} and Lemma~\ref{lem:order_stat}}
\label{app:bnd_norm}

In this appendix, we present proofs for Lemma~\ref{lem:bnd_norm} and~\ref{lem:order_stat}, respectively. \\

Our proofs rely on observation~\eqref{eqn:thm_exp_psi_3} made in Appendix~\ref{app:pf_thm}, according to which for an arbitrary deterministic multi-variate real-valued function $\Psi$, for each non-faulty agent $i$ we have
\begin{align}
    \E_{\zeta^t} \Psi\left(g^t_i\right)  = \E_{\zeta^t_i} \Psi\left(g^t_i\right). \label{eqn:lem_exp_psi_3}
\end{align}
~

For an arbitrary non-faulty agent $i$ note that
\[\E_{\zeta^t_i}\left( g^t_i \right) = \E_{\z^t_i}\left( g^t_i \right), \quad \forall t.\]
% each sampled independently and identically from the probability distribution $\D$ for computing its stochastic gradient $g^t_i$ as shown in~\eqref{eqn:avg_grad}. Let $Z^t_i = \{z^t_{i_1}, \ldots, \, z^t_{i_k}\}$. We use notation $\E_{Z^t_i}$ to denote the expectation with respect to the collective data points $Z^t_i$. 
Upon substituting $g^t_i$ from~\eqref{eqn:avg_grad} on the right hand side above we obtain that
\begin{align}
    \E_{\zeta^t_i}\left( g^t_i \right) = \left(\frac{1}{k}\right) \, \E_{\z^t}\sum_{j = 1}^k \left( \nabla \ell (w^t, \, z^t_{i_j}) \right) \label{eqn:exp_grad_0}
\end{align}
where the gradient of loss function $\ell(\cdot, \, \cdot)$ is with respect to its first argument $w$. From~\eqref{eqn:non-f_data}, recall that $\z^t$ constitutes $k$ data points that are i.i.d.~as per the probability distribution $\D$. Upon using this fact in~\eqref{eqn:exp_grad_0} we obtain that 
\begin{align}
    \E_{\zeta^t_i}\left( g^t_i \right) = \frac{1}{k} \sum_{j = 1}^k \E_{z^t_{i_j} \sim \D} \left( \nabla \ell (w^t, \, z^t_{i_j}) \right), \quad \forall t. \label{eqn:exp_grad_1}
\end{align}
Note that
\begin{align}
    \nabla Q(w) = \E_{z \sim \D} \left( \nabla \ell (w, \, z) \right), \quad \forall w \in \R^d. \label{eqn:nabla_Q}
\end{align}
Substituting from~\eqref{eqn:nabla_Q} in~\eqref{eqn:exp_grad_1} we obtain that an arbitrary non-faulty agent $i$,
\begin{align}
    \E_{\zeta^t_i}\left( g^t_i \right) = \frac{1}{k} \sum_{j = 1}^k \left(\nabla Q(w^t) \right) = \nabla Q(w^t). \label{eqn:exp_grad}
\end{align}
~

We now present a proof of Lemma~\ref{lem:bnd_norm}, followed by a proof of Lemma~\ref{lem:order_stat}.

\subsection{Proof of Lemma~\ref{lem:bnd_norm}}

Recall the lemma: \\

\noindent \fbox{\begin{minipage}{0.96\textwidth}
\begin{lemma*}[Restated]
For an arbitrary iteration $t$, if Assumption~\ref{asp:bnd_var} holds true then for each non-faulty agent $i$,
\[ \E_{\zeta^t} \norm{ g^t_i }^2 \leq \sigma^2 + \norm{\nabla Q(w^t)}^2.\]
\end{lemma*}
\end{minipage}}
~\\

\begin{proof}
Let $i$ be an arbitrary non-faulty agent. Using the definition of Euclidean norm, note that for each iteration $t$,
\begin{align}
    \norm{g^t_i - \E_{\zeta^t} \left(g^t_i\right)}^2 = \norm{g^t_i}^2 - 2 \iprod{g^t_i}{\E_{\zeta^t} \left(g^t_i\right)} + \norm{\E_{\zeta^t} \left(g^t_i\right)}^2. \label{eqn:norm_expand}
\end{align}
As the expected value of a constant is the constant itself, upon taking expectations on both sides in~\eqref{eqn:norm_expand} we obtain that
\begin{align}
    \E_{\zeta^t} \norm{g^t_i - \E_{\zeta^t} \left(g^t_i\right)}^2 = \E_{\zeta^t} \norm{g^t_i}^2 - \norm{\E_{\zeta^t} \left(g^t_i\right)}^2. \label{eqn:lem_1_zeta_1}
\end{align}
Note, from~\eqref{eqn:lem_exp_psi_3}, that
\[\E_{\zeta^t} \left(g^t_i\right) = \E_{\z^t_i} \left(g^t_i\right), \text{ and }\E_{\zeta^t} \norm{g^t_i - \E_{\zeta^t} \left(g^t_i\right)}^2 = \E_{\z^t_i} \norm{g^t_i - \E_{\z^t_i} \left(g^t_i\right)}^2.\]
Substituting the above in~\eqref{eqn:lem_1_zeta_1} we obtain that
\begin{align}
    \E_{\z^t_i} \norm{g^t_i - \E_{\z^t_i} \left(g^t_i\right)}^2 = \E_{\zeta^t} \norm{g^t_i}^2 - \norm{\E_{\z^t_i} \left(g^t_i\right)}^2. \label{eqn:lem_1_zeta_2}
\end{align}
Recall from~\eqref{eqn:exp_grad} in Section~\ref{sec:review} that $\E_{\z^t_i} ~ ( g^t_i ) = \nabla Q(w^t)$. Substituting this above we obtain that
\begin{align}
   \E_{\z^t_i} \norm{g^t_i - \E_{\z^t_i} \left(g^t_i\right)}^2 = \E_{\zeta^t} \norm{g^t_i}^2 - \norm{\nabla Q(w^t)}^2. \label{eqn:lem_1_zeta_3}
\end{align}
As Assumption~\ref{asp:bnd_var} holds true, 
\[\E_{\z^t_i} \norm{g^t_i - \E_{\z^t_i} \left(g^t_i\right)}^2 \leq \sigma^2.\]
Substituting the above in~\eqref{eqn:lem_1_zeta_3} we obtain that
\[\E_{\zeta^t} \norm{g^t_i}^2 \leq \sigma^2 + \norm{\nabla Q(w^t)}^2, \quad \forall t \geq 0.\]
As $i$ is an arbitrary non-faulty agent, the above proves the lemma. 
\end{proof}

% We now present the proof of Lemma~\ref{lem:order_stat} restated below.\\

% \section{Proof of Lemma~\ref{lem:order_stat}}
% \label{app:order_stat}
% In this appendix, we present the proof for Lemma~\ref{lem:order_stat}, restated below. \\

\subsection{Proof of Lemma~\ref{lem:order_stat} }

Recall the lemma:\\

\noindent \fbox{\begin{minipage}{0.96\textwidth}
\begin{lemma*}[Restated]
For each iteration $t$, let $\nu_t$ denote the non-faulty agent in $\H$ with stochastic gradient $g^t_{\nu_t}$ of largest Euclidean norm, that is,
\[\norm{g^t_{\nu_t}} \geq \norm{g^t_i}, \quad \forall i \in \H.\]
For an arbitrary iteration $t$, if Assumption~\ref{asp:bnd_var} holds true then
\begin{align*}
    \E_{\zeta^t} \, \norm{g^t_{\nu_t}} \leq \sigma \left( 1 + \sqrt{n-f-1} \right) + \norm{\nabla Q(w^t)}.
\end{align*}
\end{lemma*}
\end{minipage}}
~\\

\begin{proof}
We begin our proof by reviewing a generic result on the upper bounds on the expectation of highest order statistic~\cite{arnold1979bounds, bertsimas2006tight}.\\

For a positive finite integer $p$, let $R_1, \ldots, \, R_p$ be $p$ independent real-valued random variables. Consider a random variable
\[R_\nu = \max\{R_1, \ldots, \, R_p\}.\]
% Suppose that the mean $\E(R_i)$ and the variance $\E\left(R_i - \E(R_i) \right)^2$ 
Let $\E(\cdot)$ denote the mean value of a random variable. If the mean and the variance of the random variables $R_1, \ldots, \, R_p$ are identically equal to $\E(R)$ and $\var(R)$, respectively, then owing to Arnold and Groeneveld~\cite{arnold1979bounds},
\begin{align}
    \E(R_\nu) \leq \E(R) + \sqrt{\var(R) \left(p-1\right)}. \label{eqn:arnold_order_bnd}
\end{align}
Now, the proof presented below relies on the above result.\\

Consider an arbitrary iteration $t$. Recall that $\H$ comprises of only non-faulty agents, specifically $n-f$ non-faulty agents. Thus, from~\eqref{eqn:lem_exp_psi_3} we obtain that, for all $i \in \H$,
% Recall from~\eqref{eqn:zeta_collection} in Section~\ref{sec:review} that $\zeta_t = \{\zeta^t_1, \ldots, \, \zeta^t_n\}$.
% Therefore, for all $i \in \H$,
% \begin{align}
%     \E_{\zeta^t}\norm{g^t_i} = \E_{\zeta^t_1, \ldots, \, \zeta^t_n} \norm{g^t_i}. \label{eqn:lem_exp_t_1}
% \end{align}
% As $\H$ comprises only non-faulty agents,
% \begin{align}
%     \zeta_i^t = \z^t_i, \quad \forall i \in \H. \label{eqn:lem_zeta_H}
% \end{align}
% Now, given the current estimate $w^t$, recall from Section~\ref{sub:s_grad} that the stochastic gradient $g^t_i$ is a function of $\z^t_i$ for all $i \in \H$ where the random variables $\z^t_i, ~ i \in \H$ are independent and identically distributed according to distribution $\D$. This, in conjunction with~\eqref{eqn:lem_zeta_H} implies that
% \begin{align}
%     \E_{\zeta^t_1, \ldots, \, \zeta^t_n} \norm{g^t_i} = \E_{\z^t_i \sim \D} \norm{g^t_i}, \quad \forall i \in \H. \label{eqn:lem_exp_t_2}
% \end{align}
% Upon substituting from~\eqref{eqn:lem_exp_t_2} in~\eqref{eqn:lem_exp_t_1} we obtain that
\begin{align}
    \E_{\zeta^t} \norm{g^t_i}  = \E_{\z^t_i} \norm{g^t_i},  \label{eqn:lem_exp_t_3}
\end{align}
and
\begin{align}
    \E_{\zeta^t}\left(\norm{g^t_i} -  \E_{\zeta^t}\norm{g^t_i} \right)^2 = \E_{\z^t_i }\left( \norm{g^t_i} - \E_{\z^t_i}\norm{g^t_i} \right)^2. \label{eqn:lem_var_t_1}
\end{align}
% Note, recall from Section~\ref{sub:s_grad} that for each agent $i \in \H$, the stochastic gradient $g^t_i$ is a function of $w^t$ and the collection of data points $\z^t_i$.  This implies that the mean, i.e., $\E_{Z^t}\norm{g^t_i}$, and the variance, i.e., $\E_{Z^t}\left(\norm{g^t_i} -  \E\norm{g^t_i} \right)^2$, of the random variable $\norm{g^t_i}$ are also identical for all $i \in \H$. 
Now, recall from the definition of $\nu_t$ and $g^t_{\nu_t}$ that $\norm{g^t_{\nu_t}}$ is a real-valued random variable such that
\[ \norm{g^t_{\nu_t}} = \max\left\{\norm{g^t_i}, ~ i \in \H\right\}.\]
Therefore, substituting from~\eqref{eqn:lem_exp_t_3} and~\eqref{eqn:lem_var_t_1} in~\eqref{eqn:arnold_order_bnd}, we obtain that for an arbitrary agent $i \in \H$,
\begin{align}
    \E_{\zeta^t} \, \norm{g^t_{\nu_t}} \leq \E_{\z^t_i}\norm{g^t_i} + \sqrt{\E_{\z^t_i}\left(\norm{g^t_i} -  \E_{\z^t_i}\norm{g^t_i} \right)^2 \left( n-f-1\right)}. \label{eqn:lem_bnd_nu_1}
\end{align}
We now show below that
\begin{align}
    \E_{\z^t_i} \, \norm{g^t_i} \leq \sigma + \norm{\nabla Q(w^t)} ~ , \quad \forall i \in \H. \label{eqn:exp_bnd_2}
\end{align}
~

Owing to Jensen's inequality~\cite{boyd2004convex}, for all $i \in \H$,
\begin{align}
    \E_{\z^t_i} \, \norm{g^t_i} = \E_{\z^t_i} \, \sqrt{\norm{g^t_i}^2} \leq \sqrt{\E_{\z^t_i} \norm{g^t_i}^2}. \label{eqn:jen_1}
\end{align}
As Assumption~\ref{asp:bnd_var} holds true, from Lemma~\ref{lem:bnd_norm} we obtain that
\begin{align}
    \E_{\z^t_i} \, \norm{g^t_i}^2 \leq \sigma^2 + \norm{\nabla Q(w^t)}^2, \quad \forall i \in \H. \label{eqn:hon_bnd_1}
\end{align}
Substituting from~\eqref{eqn:hon_bnd_1} in~\eqref{eqn:jen_1} we obtain that
\begin{align}
    \E_{\z^t_i } \, \norm{g^t_i} \leq \sqrt{\sigma^2 + \norm{\nabla Q(w^t)}^2} ~ , \quad \forall i \in \H. \label{eqn:exp_bnd}
\end{align}
From triangle inequality, 
\[\sqrt{\sigma^2 + \norm{\nabla Q(w^t)}^2} \leq \sigma + \norm{\nabla Q(w^t)}.\]
Substituting the above in~\eqref{eqn:exp_bnd} proves~\eqref{eqn:exp_bnd_2}, i.e, 
\[\E_{\z^t_i } \, \norm{g^t_i} \leq \sigma + \norm{\nabla Q(w^t)} ~ , \quad \forall i \in \H.\]
Next, we show that 
\begin{align}
    \E_{\z^t_i}\left(\norm{g^t_i} -  \E_{\z^t_i}\norm{g^t_i} \right)^2 \leq \sigma^2  ~ , \quad \forall i \in \H. \label{eqn:exp_bnd_var_1}
\end{align}
~

Note that for all $i$,
\begin{align}
    \E_{\z^t_i}\left(\norm{g^t_i} -  \E_{\z^t_i }\norm{g^t_i} \right)^2 = \E_{\z^t_i } \norm{g^t_i}^2 - \left( \E_{\z^t_i } \norm{g^t_i} \right)^2. \label{eqn:bnd_basic_var}
\end{align}
Now, as Euclidean norm $\norm{\cdot}$ is a convex function~\cite{boyd2004convex}, using Jensen's inequality we obtain that
\begin{align}
    \E_{\z^t_i } \norm{g^t_i} \geq \norm{\E_{\z^t_i }\left(g^t_i\right)}, \quad \forall i \in \H. \label{eqn:jen_norm_1}
\end{align}
As all agents in $\H$ are non-faulty, recall from~\eqref{eqn:exp_grad} in Section~\ref{sec:review} that
\begin{align*}
    \E_{\z^t_i }\left(g^t_i\right) = \nabla Q(w^t), \quad \forall i \in \H.
\end{align*}
Upon substituting from above in~\eqref{eqn:jen_norm_1} we obtain that
\begin{align}
    \E_{\z^t_i } \norm{g^t_i} \geq \norm{\nabla Q(w^t)}, \quad \forall i \in \H. \label{eqn:jen_norm_2}
\end{align}
Substituting from~\eqref{eqn:jen_norm_2} in~\eqref{eqn:bnd_basic_var} we obtain that
\begin{align}
    \E_{\z^t_i }\left(\norm{g^t_i} -  \E_{\z^t_i }\norm{g^t_i} \right)^2 \leq \E_{\z^t_i } \norm{g^t_i}^2 - \norm{\nabla Q(w^t)}^2, \quad \forall i \in \H. \label{eqn:bnd_basic_var_2}
\end{align}
Substituting from~\eqref{eqn:hon_bnd_1} in~\eqref{eqn:bnd_basic_var_2} we obtain that
\begin{align*}
    \E_{\z^t_i }\left(\norm{g^t_i} -  \E_{\z^t_i }\norm{g^t_i} \right)^2 \leq \sigma^2 + \norm{\nabla Q(w^t)}^2 - \norm{\nabla Q(w^t)}^2 = \sigma^2, \quad \forall i \in \H. 
\end{align*}
The above proves~\eqref{eqn:exp_bnd_var_1}, i.e, 
\begin{align*}
    \E_{\z^t_i }\left(\norm{g^t_i} -  \E_{\z^t_i}\norm{g^t_i} \right)^2 \leq \sigma^2  ~ , \quad \forall i \in \H.
\end{align*}
~

Finally, substituting from~\eqref{eqn:exp_bnd_2} and~\eqref{eqn:exp_bnd_var_1} in~\eqref{eqn:lem_bnd_nu_1} we obtain that
\begin{align*}
    \E_{\zeta^t} \, \norm{g^t_{\nu_t}} & \leq \sigma + \norm{\nabla Q(w^t)} + \sqrt{\sigma^2 \left( n-f-1\right)} \\
    & = \sigma \left(1 + \sqrt{n-f-1} \right) + \norm{\nabla Q(w^t)}.
\end{align*}
As $t$ above is an arbitrary iteration, the above proves the lemma.
\end{proof}

\end{document}
