# Supplementary material for: Byzantine Fault-Tolerant Distributed Machine Learning Using Stochastic Gradient Descent (SGD) and Norm-Based Comparative Gradient Elimination (CGE)
Source: arXiv:2008.04699 source file (2021-04-18)
Supplement: Supplementary file 5 [file appendix_experiments_backup.tex]

\iffalse
\subsection{Experiments on gradient averaging scheme}
\label{sub:appendix_averaging}

We noticed that in previous experimental results, there are `unstable' behaviors shown in the plots, especially when under the fault type of \textit{coordinate-wise}. We can see that in some cases, for example, $f=0$ or $1$ in Figure~\ref{fig:fault-fraction-1}(b), that the minimums of loss during the training process can be very close to the corresponding fault-free loss, there are pikes and turbulence once several steps. To address this problem, one possible way is to increase batch size. As is shown in Figure~\ref{fig:fault-fraction-3}(b), when batch size is increased from 16 to 64, although the pikes still exists, it become smaller and less frequent, thanks to the reduce of variance of the gradients.

Another way of address this problem might be using a gradient averaging scheme. By averaging previous steps gradients collected from each agent, it is expected to reduce variance among good agents, so that gradients from fault agents become more distinguishing to filters. Let $h^t_j$ denote the averaging history of gradients of agent $t$ at step $j$, $0\leq\alpha\leq1$,
$$h^t_j = \alpha\cdot h^{t-1}_j + (1-\alpha) g^t_j$$
Update parameters by the following scheme instead of:
$$w^t = w^{t-1} + \mu\cdot\mathrm{Filter}_j\{h^t_j\}$$
Note that under this definition, $\alpha=0$ indicates plain SGD with no averaging.

We conducted several experiments with averaging scheme described above. Figure~\ref{fig:accumulation-1} and Figure~\ref{fig:accumulation-2} shows the results. The value of $\alpha$ varies between 0 and 0.60. Comparing plots in each figure, it is easy to find that with an increase of the value of $\alpha$, the pike in loss (or dive in precision) become less significant and less frequent. Also, convergence speed does not change much with increasing of $\alpha$. In Figure~\ref{fig:accumulation-1}(b), we see that this averaging scheme can sometimes also helps SGD avoid a worse local minimum.

One thing worth noticing is that, the averaging scheme does not increase computation complexity by much.

\begin{figure}[t]
    \centering
    \includegraphics[width=\textwidth]{Experiments/new/accumulation_comparison/averaging-comparison-1.pdf}
    \caption{Comparison of different $\alpha$ values using averaging scheme, using filter multi-KRUM ($m=2$) with batch size 16, under fault type \textit{coordinate-wise}. Each row correspond to a different number of faults: (a) $f=1$, (b) $f=2$, (c) $f=3$, and (d) $f=4$.}
    \label{fig:accumulation-1}
\end{figure}

\begin{figure}[t]
    \centering
    \includegraphics[width=\textwidth]{Experiments/new/accumulation_comparison/averaging-comparison-2.pdf}
    \caption{Comparison of different $\alpha$ values using averaging scheme, using filter CGE with batch size 16, under fault type \textit{coordinate-wise}. Each row correspond to a different number of faults: (a) $f=1$, (b) $f=2$, (c) $f=3$, and (d) $f=4$.}
    \label{fig:accumulation-2}
\end{figure}

\subsection{Experiments on CIFAR-10}

We conducted several experiments in a different dataset, CIFAR-10\cite{krizhevsky2009learning}. CIFAR-10, similar to MNIST, is also an image-classification dataset. It consists of 60,000 color images in 10 mutually exclusive categories, \emph{e.g.} automobile, bird, dog, etc., with equal number of images in each class. The dataset is further divided into a training set of 50,000 samples and a testing set with 10,000 samples. Classification in CIFAR-10 is expected to be a more difficult task comparing to that in MNIST, since images in MNIST are monochrome and with less variety, while classes in CIFAR-10 can be vague: sedan and SUV can both be automobile, or dogs can have many breeds that look very different. We train models using SGD on LeNet for classification task of CIFAR-10, with 10 agents in parallel, out of them $f$ are fault agents.

Some of the results are documented here in Figure~\ref{fig:cifar-1}. As CIFAR-10 is a more difficult task to MNIST and we are using the same neural network, we see that the speed of convergence is much slower than what we have in MNIST, and with the same 300 steps, we can only see a trend of convergence. But still, some filters works better than others. Geometric median (a), median of means (b), and coordinate-wise trimmed mean (c) cannot handle the case where there are 4 out of 10 fault agents. There is a gap between multi-KRUM plots and fault-free plot, while CGE, out of the five filters, help SGD converge with a speed close to the fault-free case.

\begin{figure}[t]
    \centering
    \includegraphics[width=\textwidth]{Experiments/new/cifar_comparison/cifar-filter-comparison-1.pdf}
    \caption{Comparison of filters when training for CIFAR-10 dataset, using batch size 16, under fault type \textit{coordinate-wise}. Each row correspond to a different filter: (a) geometric median, (b) median of means, (c) coordinate-wise trimmed mean, (d) multi-KRUM ($m=2$), and (e) CGE.}
    \label{fig:cifar-1}
\end{figure}

Similarly to what we do in Appendix \ref{sub:appendix_averaging}, we can also apply averaging scheme on CIFAR-10 tasks, where due to the variety of training samples, the variance of gradients would be even higher than in MNIST. Figures~\ref{fig:cifar-accumulation-1} and \ref{fig:cifar-accumulation-2} presents the results. Comparing to plots in Figure~\ref{fig:cifar-1}(d) and \ref{fig:cifar-1}(e), we see that the turbulence also reduces when value of $\alpha$ increases, regardless of the filter. We also notice that there is a small gap between plots of multi-KRUM and the fault-free plot, while averaging would further help CGE eliminate that gap.

\begin{figure}[t]
    \centering
    \includegraphics[width=\textwidth]{Experiments/new/cifar_comparison/cifar-averaging-comparison-1.pdf}
    \caption{Comparison of different $\alpha$ values using averaging scheme when training for CIFAR-10 dataset, using filter multi-KRUM ($m=2$) with batch size 16, under fault type \textit{coordinate-wise}. Each row correspond to a different number of faults: (a) $f=1$, (b) $f=2$, (c) $f=3$, and (d) $f=4$.}
    \label{fig:cifar-accumulation-1}
\end{figure}

\begin{figure}[t]
    \centering
    \includegraphics[width=\textwidth]{Experiments/new/cifar_comparison/cifar-averaging-comparison-2.pdf}
    \caption{Comparison of different $\alpha$ values using averaging scheme when training for CIFAR-10 dataset, using filter CGE with batch size 16, under fault type \textit{coordinate-wise}. Each row correspond to a different number of faults: (a) $f=1$, (b) $f=2$, (c) $f=3$, and (d) $f=4$.}
    \label{fig:cifar-accumulation-2}
\end{figure}
\fi
